# Supplementary material for: On Diffusion Process in SE(3)-invariant Space
Source: arXiv:2403.01430 source file (2024-03-03)
Supplement: Supplementary file 1 [file vismol.tex]

\begin{figure}[tb]
    \centering
    \begin{tabular}{cc}
    Method &QM9 \\

    \makecell{2D} & \raisebox{-.4\totalheight}{\includegraphics[width=.45\textwidth]{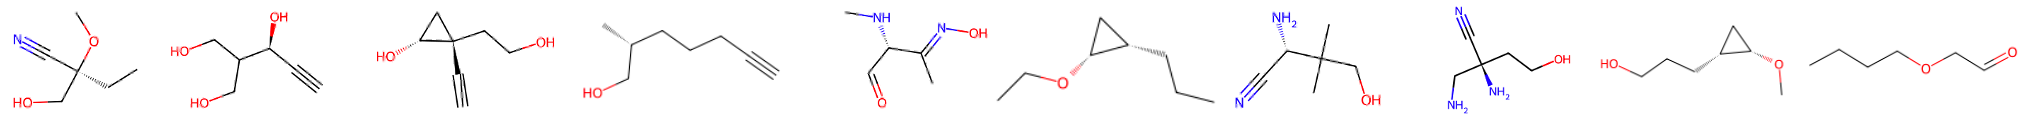}} \\
    \makecell{SDE\\1000} & \raisebox{-.4\totalheight}{\includegraphics[width=.45\textwidth]{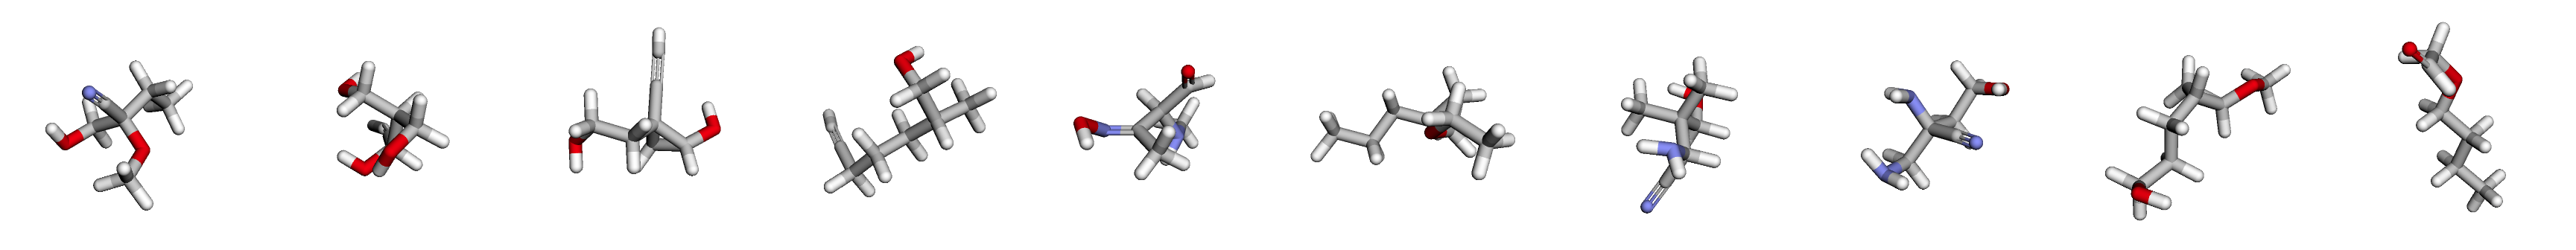}} \\
    \makecell{SDE\\100} & \raisebox{-.4\totalheight}{\includegraphics[width=.45\textwidth]{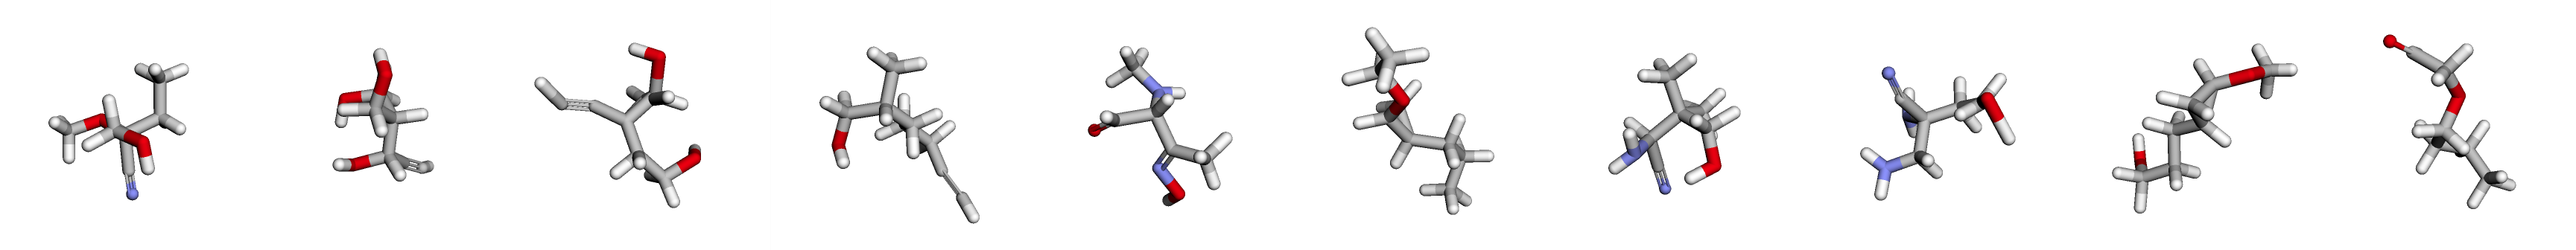}} \\
    \makecell{ODE\\1000} &  \\
    \makecell{ODE\\100} & \raisebox{-.4\totalheight}{\includegraphics[width=.45\textwidth]{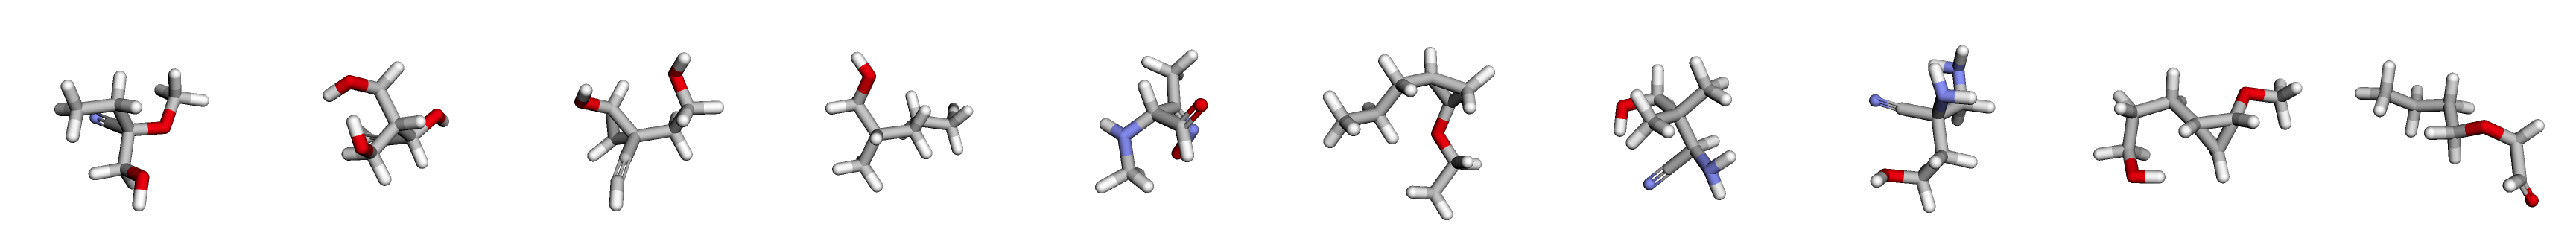}} \\

    \makecell{2D} & \raisebox{-.4\totalheight}{\includegraphics[width=.45\textwidth]{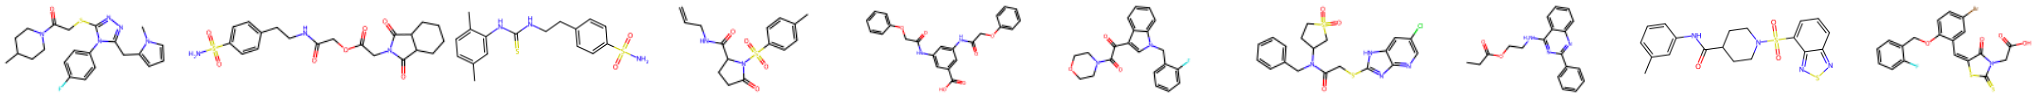}} \\
    \makecell{SDE\\1000} & \raisebox{-.4\totalheight}{\includegraphics[width=.45\textwidth]{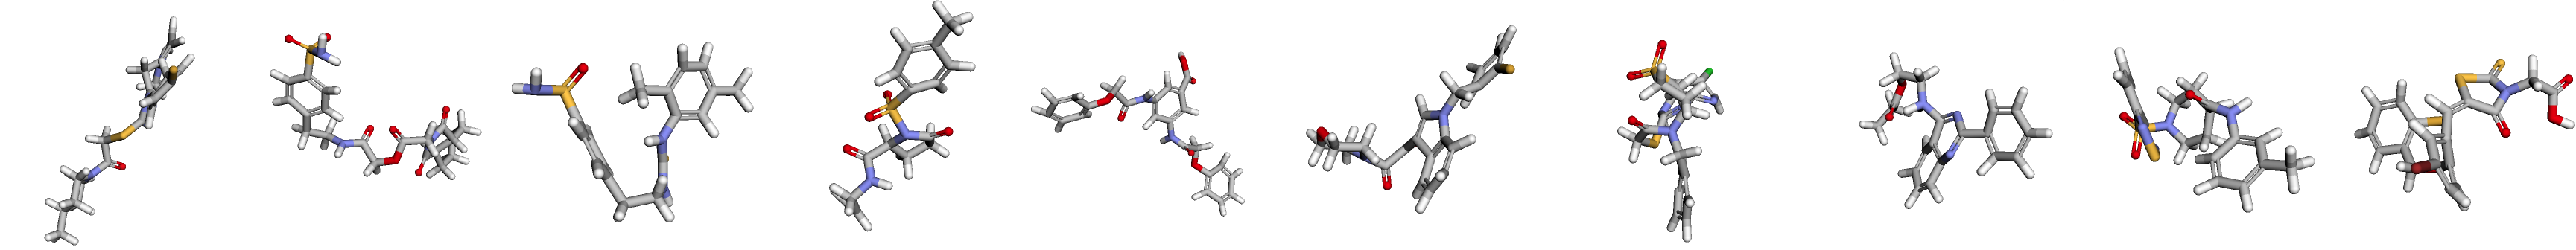}} \\
    \makecell{SDE\\100} & \raisebox{-.4\totalheight}{\includegraphics[width=.45\textwidth]{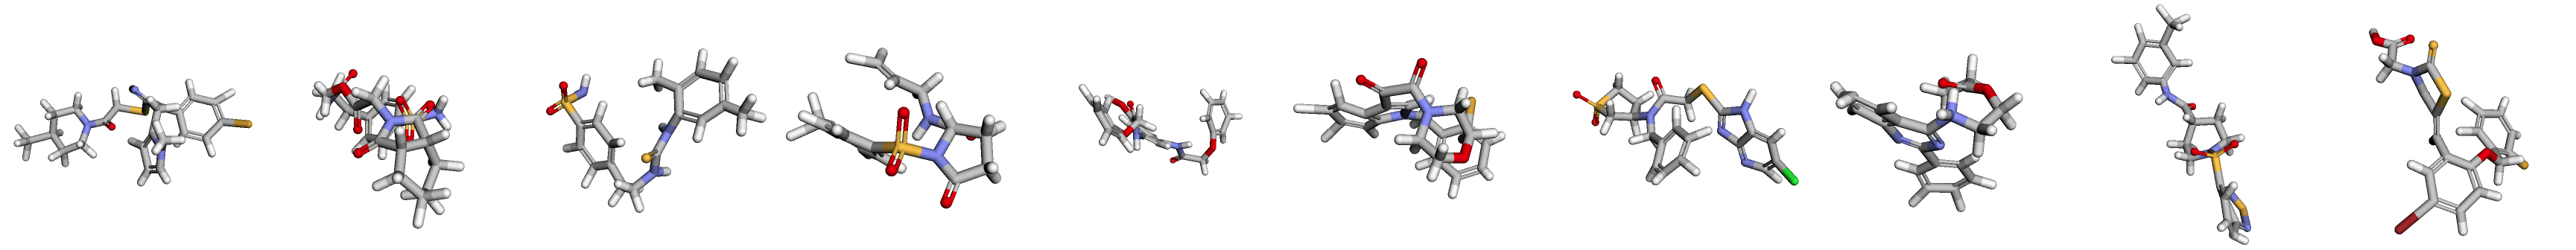}} \\
    \makecell{ODE\\1000} &  \\
    \makecell{ODE\\100} & \raisebox{-.4\totalheight}{\includegraphics[width=.45\textwidth]{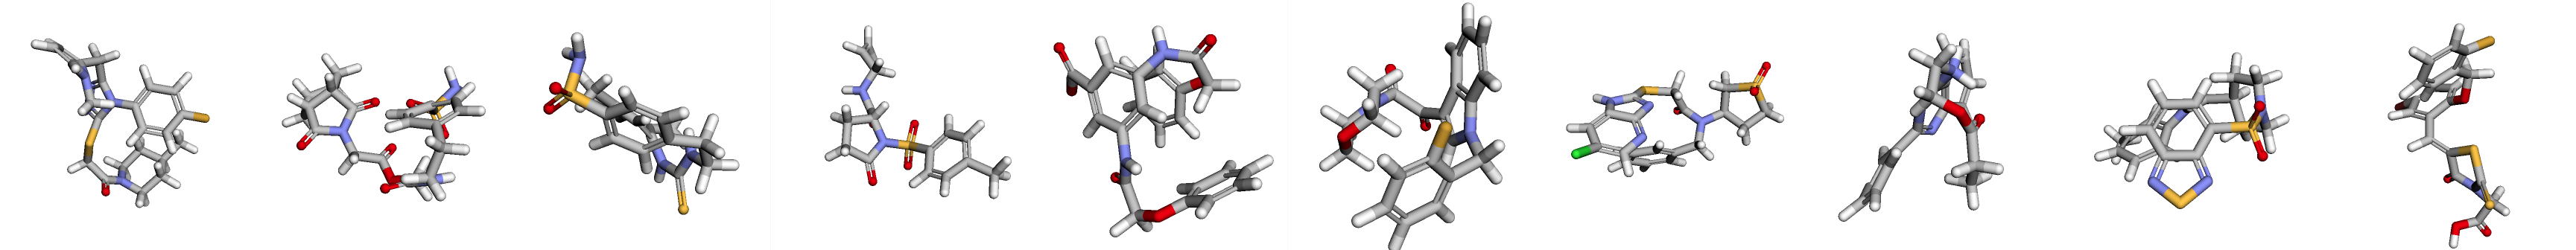}} \\

    \label{fig: vis-mol}
    \end{tabular}
    \caption{mol vis}
\end{figure}

% \begin{figure}[tb]
%     \centering
%     \begin{tabular}{c c}
%     \makecell{ODE\\100} & \raisebox{-.4\totalheight}{\includegraphics[width=.8\textwidth]{appendix/mol_vis/vis-mol-drugs-ode-100.png}} \\
%     \makecell{ODE\\1000} & \raisebox{-.4\totalheight}{\includegraphics[width=.8\textwidth]{appendix/mol_vis/vis-mol-drugs-ode-1000.png}} \\
%     \makecell{SDE\\100} & \raisebox{-.4\totalheight}{\includegraphics[width=.8\textwidth]{appendix/mol_vis/vis-mol-drugs-sde-100.png}} \\
%     \makecell{SDE\\1000} & \raisebox{-.4\totalheight}{\includegraphics[width=.8\textwidth]{appendix/mol_vis/vis-mol-drugs-sde-1000.png}}\\
%     \makecell{Naive ODE\\100} & \raisebox{-.4\totalheight}{\includegraphics[width=.8\textwidth]{appendix/mol_vis/vis-mol-drugs-naiveode-100.png}} 
%     \label{fig: sde-25}
%     \end{tabular}
%     \caption{mol traj}
% \end{figure}
