# Supplementary material for: On Diffusion Process in SE(3)-invariant Space
Source: arXiv:2403.01430 source file (2024-03-03)
Supplement: Supplementary file 2 [file vistraj.tex]

\begin{figure}[h]
    \centering
    \begin{tabular}{c c}
    \makecell{Methods \\/ Steps} & $\xrightarrow{\text{{\small Noise}}\hspace*{13cm}\text{{\small Molecule}}}$ \\
    & \includegraphics[width=.08\textwidth]{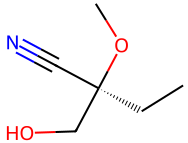} \\
    \makecell{ODE\\100} & \raisebox{-.4\totalheight}{\includegraphics[width=.9\textwidth]{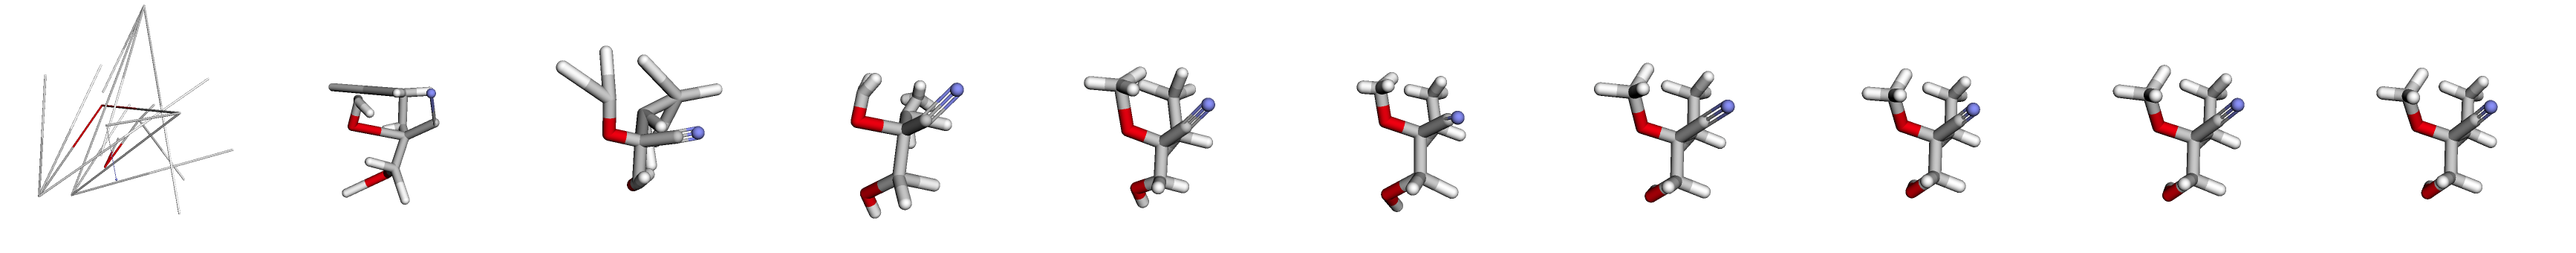}} \\
    \makecell{ODE\\1000} & \raisebox{-.4\totalheight}{\includegraphics[width=.9\textwidth]{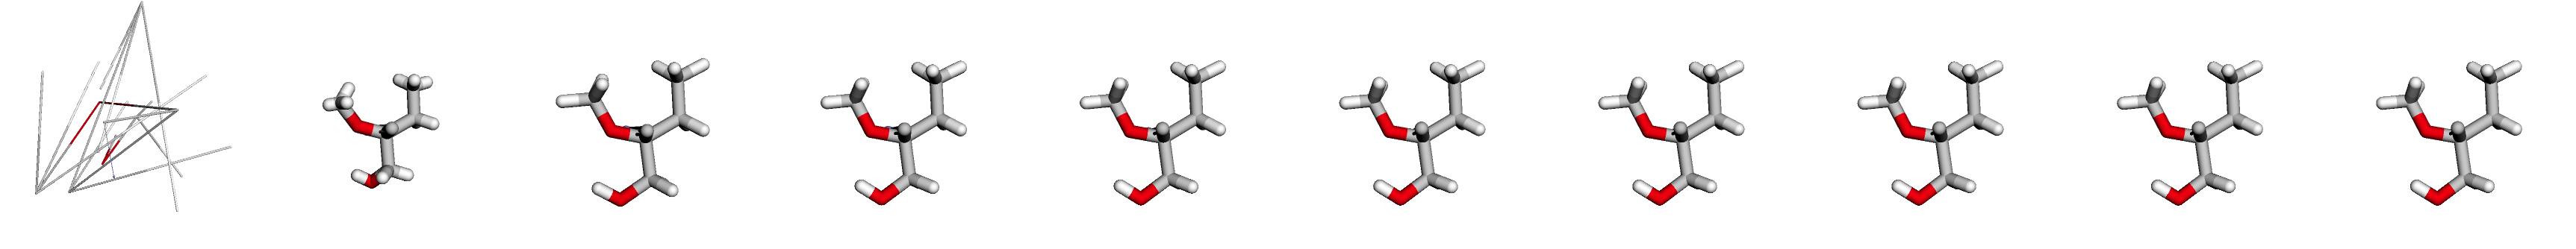}} \\
    \makecell{SDE\\100} & \raisebox{-.4\totalheight}{\includegraphics[width=.9\textwidth]{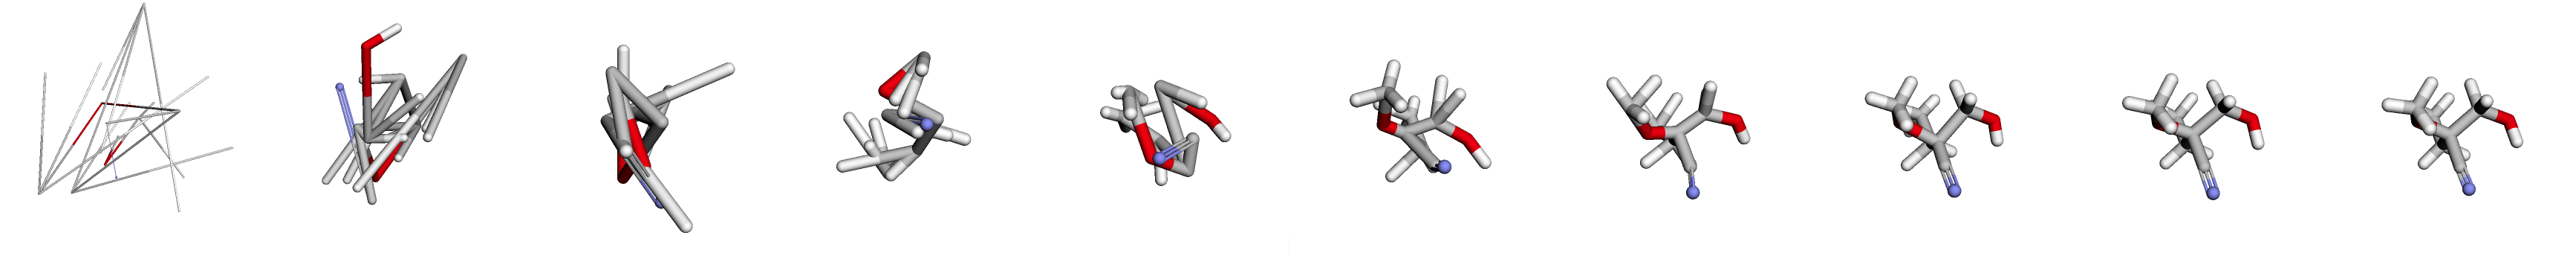}} \\
    \makecell{SDE\\1000} & \raisebox{-.4\totalheight}{\includegraphics[width=.9\textwidth]{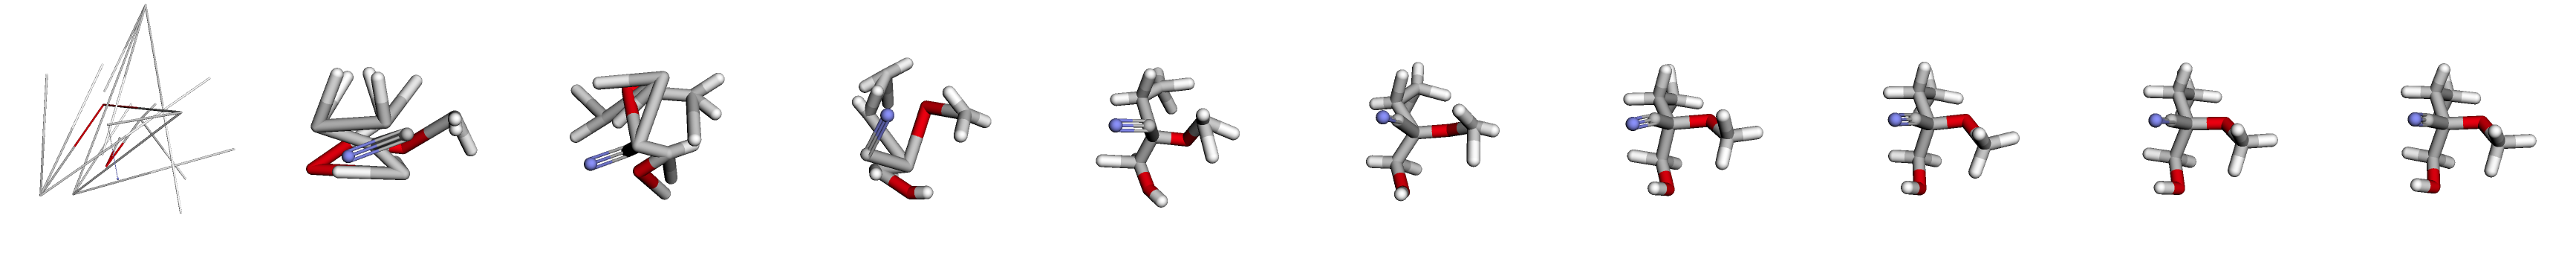}} \\
    \makecell{Naive ODE\\100} & \raisebox{-.4\totalheight}{\includegraphics[width=.9\textwidth]{appendix/mol_vis/vistraj-qm9-naiveode-100.png}} 
    \label{fig: traj-qm9}
    \end{tabular}
    \caption{mol traj}
\end{figure}

\begin{figure}[h]
    \centering
    \begin{tabular}{c c}
    \makecell{Methods \\/ Steps} & $\xrightarrow{\text{{\small Noise}}\hspace*{13cm}\text{{\small Molecule}}}$ \\
    % & \includegraphics[width=.1\textwidth]{appendix/mol_vis/vis-traj-drugs-2D.png} \\
    \makecell{ODE\\100} & \raisebox{-.4\totalheight}{\includegraphics[width=.9\textwidth]{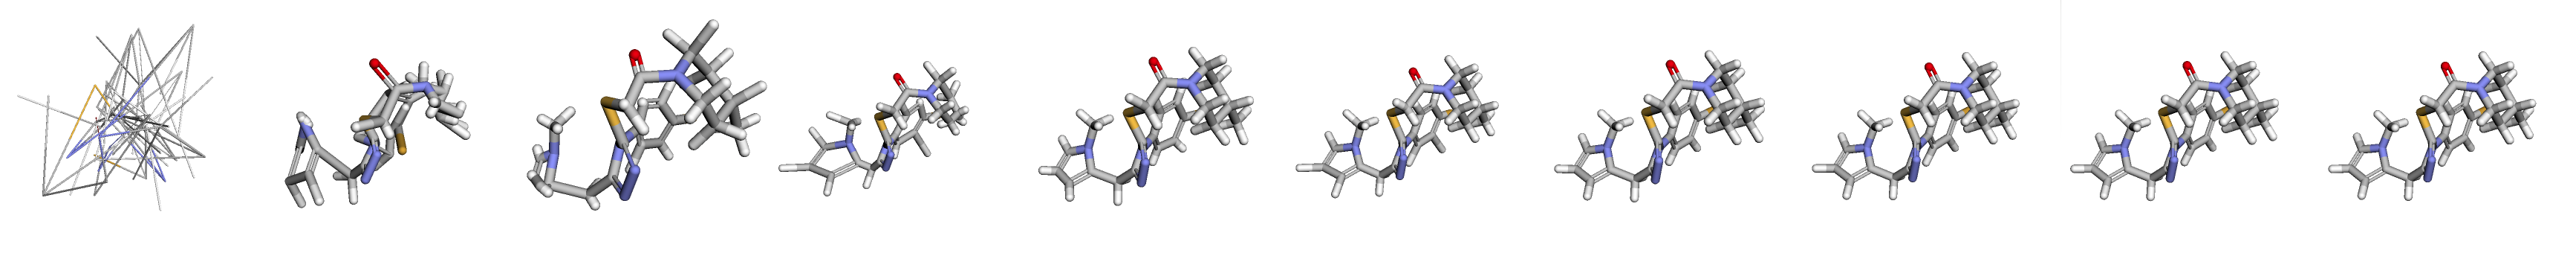}} \\
    \makecell{SDE\\100} & \raisebox{-.4\totalheight}{\includegraphics[width=.9\textwidth]{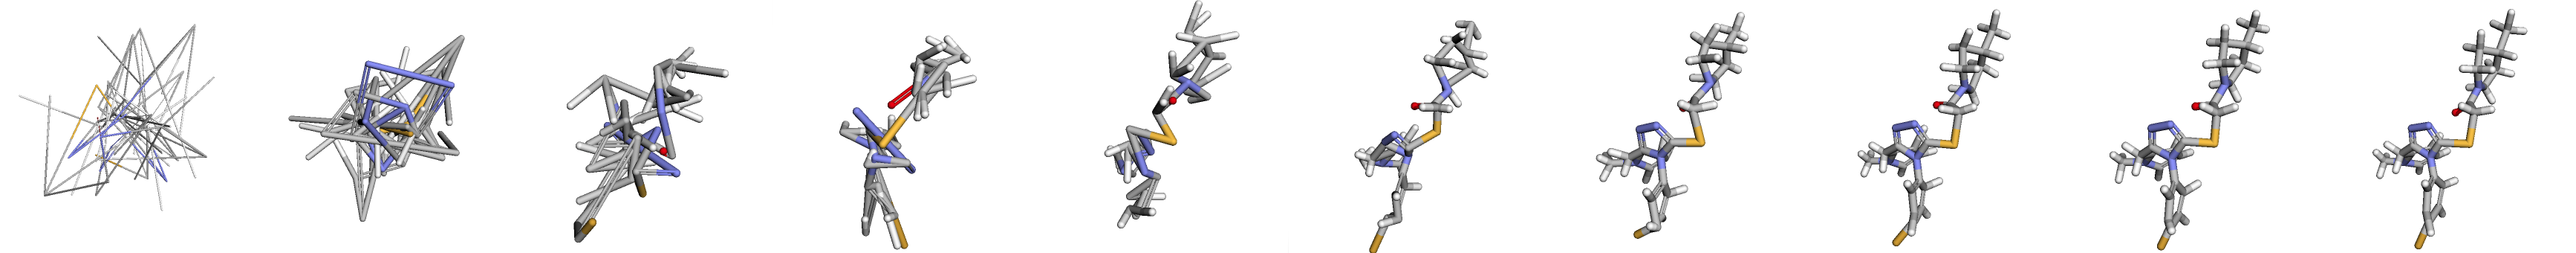}} \\
    \makecell{Naive ODE\\100} & \raisebox{-.4\totalheight}{\includegraphics[width=.9\textwidth]{appendix/mol_vis/vistraj-drugs-naiveode-100.png}} \\
    \makecell{ODE\\1000} & \raisebox{-.4\totalheight}{\includegraphics[width=.9\textwidth]{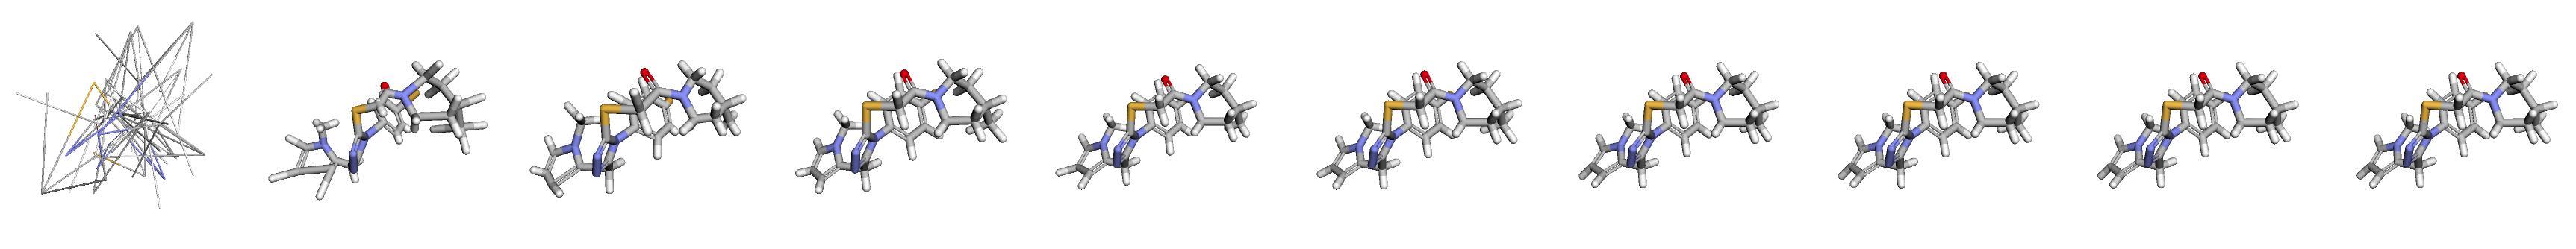}} \\
    \makecell{SDE\\1000} & \raisebox{-.4\totalheight}{\includegraphics[width=.9\textwidth]{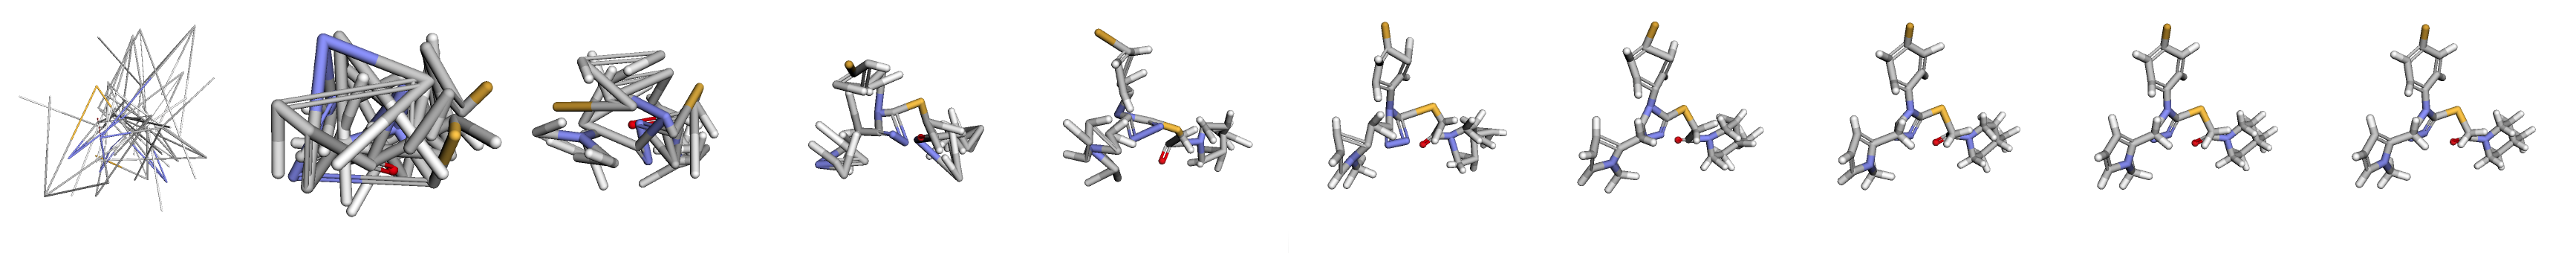}}\\
    \label{fig: traj-drugs}
    \end{tabular}
    \caption{mol traj}
\end{figure}
